# Supplementary material for: GradOrth: A Simple yet Efficient Out-of-Distribution Detection with Orthogonal Projection of Gradients
Source: arXiv:2308.00310 source file (2023-08-01)
Supplement: Supplementary file 1 [file appendix.tex]

\textbf{Convolutional Layer}
The convolutional layer includes filters that operate in a different way on the inputs than the weights in a fully connected (FC) layer. We present the input tensor by $\mathcal{X} \in \R^{C_i \times h_i \times \theta_i}$ and filters by $\mathcal{\theta} \in \R^{C_o \times C_i \times k \times k}$ in a convolutional layer. The convolution on $\langle \mathcal{X},\mathcal{\theta},*\rangle$ produces output feature map, $\mathcal{O} \in \R^{C_o \times h_o \times \theta_o}$ ~\citep{conv_op}. We present the number of input/output channels of the Convolutional layer by $C_i$/$C_o$. We also leverage $h_i$, $\theta_i$ ($h_o$, $\theta_o$) to denote the height and width of the input (output) feature maps and $k$ is the filters kernel size. As shown in Figure~\ref{fig:fig1}(a), if $\mathcal{X}$ is reshaped into a $(h_o \times \theta_o) \times (C_i\times k \times k)$ matrix, $\mX$ and $\mathcal{W}$ is reshaped into a $(C_i\times k \times k) \times C_o $ matrix, $\m\theta$, then the convolution can be expressed as matrix multiplication between $\mX$ and $\m\theta$ as $\mO$=$\mX\m\theta$, where $\mO \in \R^{(h_0\times \theta_0)\times C_o}$. Each row of $\mX$ contains an input patch vector, $\vp_j \in \R^{(C_i\times k \times k) \times 1}$, where $j=1,2...,n$ $(n=h_o*\theta_o)$.

By expressing convolution as a matrix multiplication, an intuitive description of gradient computation can be presented during backpropagation. In Convolutional layer, during backward pass an error matrix $\bm{\Delta}$ of size $(h_0\times \theta_0)\times C_o$ (same size as $\mO$) is computed from the next layer, Similar to the Fully-Connected layer case. therefore, the gradient of loss with respect to filter weights is derived by 
\begin{equation}
    \nabla_{\mW} L = \mX^T \bm{\Delta},  
\end{equation}
where, $\nabla_{\m\theta}L$ is of shape $(C_i\times k \times k) \times C_o $ (same size as $\m\theta$). The gradient updates of the convolutional filters will lie in the space spanned by the input patch vectors ($\vp$) Since columns of $\mX^T$ are the input patch vectors ($\vp$).
